# Supplementary material for: Feedback effect on the observable properties of $z>6$ AGN
Source: arXiv:2205.09181 source file (2022-05-18)
Supplement: Supplementary file 1 [file additional_def.tex]

% element astro-like

%
%\def\CIIion{\hbox{C~$\scriptstyle\rm II $}}
%\def\OIion{\hbox{O~$\scriptstyle\rm I $}}
%\def\OIIIion{\hbox{O~$\scriptstyle\rm III $}}
%\def\NIIion{\hbox{O~$\scriptstyle\rm II $}}
%

% FIR emission lines

% absorption lines

% mnras style for code names

% cosmo

%

% math

% chemistry
\def\nh2{n_{\rm H2}}
\def\fh2{f_{\rm H2}}

% units

\def\angstrom{\textrm{A\kern -1.3ex\raisebox{0.6ex}{$^\circ$}}}

% solar stuff

%

%

%

%lum and ions

% additional convenience stuff

% names shortcuts
